# Supplementary material for: Large Language Models for In-Context Student Modeling: Synthesizing Student's Behavior in Visual Programming
Source: arXiv:2310.10690 source file (2024-05-03)
Supplement: Supplementary file 1 [file 8_appendix.tex]

% !TEX root =  main.tex
%%%%%%%%%%%%%%%%%%%%%%%%%%%%%%%%%%%
%%%%%%%%%%%%%%%%%%%%%%%%%%%%%%%%%%%
\clearpage
\appendix
\section{Experiments in Python Programming}
\begin{figure}[!h]
    \centering
    \includegraphics[width=0.95\textwidth]{arXiv/figs/appendix/python_problem_setup.pdf}
    \vspace{0.1cm}
    \caption{Illustration of our problem setup in Python programming. The scenario is taken from \cite{DBLP:conf/icer/PhungPCGKMSS22}. A synthesizer observes a student \student's misconception. Then, given a target task $T^{\tar}$, the synthesizer generates a student's attempt $\widehat{C}^{\student}_{T^{\tar}}$ that imitates the student's behavior.}
    \label{fig:python-problem-setup}
\end{figure}

\begin{figure}[!h]    
    \centering
    \scalebox{0.8}{
    \setlength\tabcolsep{5pt}
    
        \begin{tabular}{|p{1.00\linewidth}|}
        \hline
        % \centerline{\color{promptheadercolor}\textnormal{Domain Background}}    
            \centerline{\color{promptheadercolor}\textnormal{Instruction}}
            
            You are a student working in the Python programming domain. Below, I give you a target task and a student's misconception. You are going to play the role of the given student and synthesize a buggy program for the target task that reflects the misconception. Additionally, synthesize a correct solution program for the target task.

            \centerline{\color{promptheadercolor}\textnormal{ Student's Context}}

             --- Student's misconception ---
            
            {\color{promptinputcolor}\{student\_misconception\}} 
            
            % --- Reference Task: Representation ---

            % {\color{promptinputcolor}\{reference\_task\_representation\}}
            
            % --- Reference Task: Solution ---
            
            % {\color{promptinputcolor}\{reference\_task\_solution\}}
            
            % --- Reference Task: Student's attempt ---
            
            % {\color{promptinputcolor}\{reference\_task\_student\_attempt\}}\newline

            \centerline{\color{promptheadercolor}\textnormal{Target Task}}
            
            --- Target Task: Description in JSON format ---
            
            {\color{promptinputcolor}\{target\_task\_description\}}\newline 

            --- Target Task: Student's buggy program ---

            \vspace{0.2cm}
            
            --- Target Task: Correct solution program ---
            \vspace{0.2cm}
        \\
        \hline
        \end{tabular}
    }
    \caption{Prompt template used in LLM-SS framework for Python programming. {\color{promptinputcolor}\{placeholders\}} are used to include details for each scenario.}
\end{figure}

\begin{figure}[!h]
    \centering
    \input{arXiv/figs/appendix/python_table_results}
    \caption{\looseness-01 Average results on all tasks, w.r.t. to each attribute in the quality rubric}
    \label{fig:python-result-details}
\end{figure}

\begin{figure}[!h]
    \centering
    \includegraphics[width=1\textwidth]{arXiv/figs/appendix/python_q_overall.pdf}
    \caption{\textsc{Q-overall} scores.}
\end{figure}

\begin{figure}[!h]
    \centering % Center the subfigures horizontally
    \begin{subfigure}{0.9\textwidth} 
    \begin{framed}
        \begin{lstlisting}[xleftmargin=.05\textwidth,language=Python]
def isPalindrome(S):
    for i in range(len(S)//2):
        if S[i] != S[len(S)-i-1]:
            return 0
    return 1\end{lstlisting}
    \end{framed}
        \caption{A solution code\\ (\textsc{Q-stu} $= 0$, \textsc{Q-task} $= 1$, \textsc{Q-overall} $= 0$)} 
        \vspace{0.5cm}
    \end{subfigure}
    \begin{subfigure}{0.9\textwidth} 
    \begin{framed}
        \begin{lstlisting}[xleftmargin=.05\textwidth,language=Python, escapechar=|]
def isPalindrome(S):
    n = len(S)
    for i in range(n//2):
        |\colorbox{pink}{if S[i] != S[-i]:}|
            return 0
    return 1\end{lstlisting}
    \end{framed}
        \caption{GPT-3.5-SS\\ (\textsc{Q-stu} $= 0.5$, \textsc{Q-task} $= 1$, \textsc{Q-overall} $= 0.5$)} 
        \vspace{0.5cm}
    \end{subfigure}
    \begin{subfigure}{0.9\textwidth} 
    \begin{framed}
        \begin{lstlisting}[xleftmargin=.05\textwidth,language=Python, escapechar=|]
def isPalindrome(S):
    length = len(S)
    for i in range(length//2):
        |\colorbox{pink}{if S[i] != S[length - i]:}|
            |\colorbox{pink}{return False}|
    |\colorbox{pink}{return True}|\end{lstlisting}
    \end{framed}
        \caption{GPT-4-SS\\ (\textsc{Q-stu} $= 1$, \textsc{Q-task} $= 1$, \textsc{Q-overall} $= 1$)} 
        \vspace{0.5cm}
    \end{subfigure}
    \begin{subfigure}{0.9\textwidth}
    \begin{framed}
        \begin{lstlisting}[xleftmargin=.05\textwidth,language=Python]
def isPalindrome(S):
    for i in range(len(S)):
        if S[i]!= S[len(S)-i-1]:
            return 0
    return 1\end{lstlisting}
    \end{framed}
    \caption{Llama2-7B-SS\\ (\textsc{Q-stu} $= 0$, \textsc{Q-task} $= 1$, \textsc{Q-overall} $= 0$)} 
    \vspace{0.5cm}
    \end{subfigure}
    \begin{subfigure}{0.9\textwidth} 
    \begin{framed}
        \begin{lstlisting}[xleftmargin=.05\textwidth,language=Python, escapechar=|]
def isPalindrome(S):
    |\colorbox{pink}{return len(S) \% 2 == 0}|\end{lstlisting}
    \end{framed}
    \caption{Llama2-70B-SS\\ (\textsc{Q-stu} $= 0.5$, \textsc{Q-task} $= 0$, \textsc{Q-overall} $= 0$)} 
    \end{subfigure}
    \caption{Student \student's attempts synthesized by different methods instantiated from our framework for the scenario shown in Figure \ref{fig:python-problem-setup}. The student's misconception is: ``\textit{There is an issue with string indexing. Return type is incorrect.}''. For each method, we show the score of each attribute in the quality rubric. We highlight lines of code that reflect the student's misconception in \colorbox{pink}{pink}.} 
\end{figure}

\begin{figure}[!h]
    \centering % Center the subfigures horizontally
    \begin{subfigure}{0.9\textwidth} 
    \begin{framed}
        \begin{lstlisting}[xleftmargin=.05\textwidth,language=Python]
def gcd(A, B):
    if A < B:
        A, B = B, A
    while(B):
        A, B = B, A % B
    return A\end{lstlisting}
    \end{framed}
        \caption{A solution code (\textsc{Q-stu} $= 0$, \textsc{Q-task} $= 1$, \textsc{Q-overall} $= 0$)} 
        \vspace{0.5cm}
    \end{subfigure}
    \begin{subfigure}{0.9\textwidth} 
    \begin{framed}
        \begin{lstlisting}[xleftmargin=.05\textwidth,language=Python, escapechar=|]
def gcd(A, B):
    if B == 0:
        return A
    else:
        return gcd(B, A%B)\end{lstlisting}
    \end{framed}
        \caption{GPT-3.5-SS (\textsc{Q-stu} $= 0$, \textsc{Q-task} $= 1$, \textsc{Q-overall} $= 0$)} 
        \vspace{0.5cm}
    \end{subfigure}
    \begin{subfigure}{0.9\textwidth} 
    \begin{framed}
        \begin{lstlisting}[xleftmargin=.05\textwidth,language=Python, escapechar=|]
def gcd(A, B):
    if B == 0:
        return A
    else:
        |\colorbox{pink}{return gcd(A, A \% B)}|\end{lstlisting}
    \end{framed}
        \caption{GPT-4-SS (\textsc{Q-stu} $= 1$, \textsc{Q-task} $= 1$, \textsc{Q-overall} $= 1$)} 
        \vspace{0.5cm}
    \end{subfigure}
    \begin{subfigure}{0.9\textwidth}
    \begin{framed}
        \begin{lstlisting}[xleftmargin=.05\textwidth,language=Python, escapechar=|]
def gcd(A, B):
    if B == 0:
        return A
    else:
        return gcd(B, A % B)\end{lstlisting}
    \end{framed}
    \caption{Llama2-7B-SS (\textsc{Q-stu} $= 0$, \textsc{Q-task} $= 1$, \textsc{Q-overall} $= 0$)} 
    \vspace{0.5cm}
    \end{subfigure}
    \begin{subfigure}{0.9\textwidth} 
    \begin{framed}
         \begin{lstlisting}[xleftmargin=.05\textwidth,language=Python, escapechar=|]
def gcd(a, b):
    if b == 0:
        return a
    else:
        |\colorbox{pink}{return gcd(b, a)}|\end{lstlisting}
    \end{framed}
    \caption{Llama2-70B-SS (\textsc{Q-stu} $= 1$, \textsc{Q-task} $= 1$, \textsc{Q-overall} $= 1$)} 
    \end{subfigure}
    \caption{Student \student's attempts synthesized by different methods instantiated from our framework for the scenario shown in Figure \ref{fig:python-problem-setup}. The student's misconception is: ``\textit{Wrong arguments are passed to the recursive function call.}''. For each method, we show the score of each attribute in the quality rubric. We highlight lines of code that reflect the student's misconception in \colorbox{pink}{pink}.} 
\end{figure}

\begin{figure}[!h]
    \centering % Center the subfigures horizontally
    \begin{subfigure}{0.9\textwidth} 
    \begin{framed}
        \begin{lstlisting}[xleftmargin=.05\textwidth,language=Python]
def nFibonacci(N):
    fibonacci_series = []
    a, b = 0, 1
    while a <= N:
        fibonacci_series.append(a)
        a, b = b, a + b
    return fibonacci_series\end{lstlisting}
    \end{framed}
        \caption{GPT-3.5-SS\\ (\textsc{Q-stu} $= 0$, \textsc{Q-task} $= 1$, \textsc{Q-overall} $= 0$)} 
        \vspace{0.5cm}
    \end{subfigure}
    \begin{subfigure}{0.9\textwidth} 
    \begin{framed}
        \begin{lstlisting}[xleftmargin=.05\textwidth,language=Python, escapechar=|]
def nFibonacci(N):
    def fib(n):
        if n <= 1:
            return n
        else:
            |\colorbox{pink}{return fib(n-1) + fib(n-2)}|
    
    fibonacci_sequence = []
    i = 0
    while True:
        fibonacci_number = fib(i)
        if fibonacci_number <= N:
            fibonacci_sequence.append(fibonacci_number)
            i += 1
        else:
            break
    return fibonacci_sequence\end{lstlisting}
    \end{framed}
        \caption{GPT-4-SS\\ (\textsc{Q-stu} $= 1$, \textsc{Q-task} $= 1$, \textsc{Q-overall} $= 1$)} 
        \vspace{0.5cm}
    \end{subfigure}
    \begin{subfigure}{0.9\textwidth}
    \begin{framed}
        \begin{lstlisting}[xleftmargin=.05\textwidth,language=Python, escapechar=|]
def nFibonacci(N):
    if N <= 1:
        return [1, 1]
    else:
        |\colorbox{pink}{return nFibonacci(N-1) + nFibonacci(N-2)}|\end{lstlisting}
    \end{framed}
    \caption{Llama2-7B-SS\\ (\textsc{Q-stu} $= 1$, \textsc{Q-task} $= 0$, \textsc{Q-overall} $= 0$)} 
    \vspace{0.5cm}
    \end{subfigure}
    \begin{subfigure}{0.9\textwidth} 
    \begin{framed}
         \begin{lstlisting}[xleftmargin=.05\textwidth,language=Python]
def nFibonacci(N):
    fib = [0, 1]
    for i in range(2, N+1):
        fib.append(fib[i-1] + fib[i-2])
    return fib\end{lstlisting}
    \end{framed}
    \caption{Llama2-70B-SS\\ (\textsc{Q-stu} $= 0$, \textsc{Q-task} $= 0.5$, \textsc{Q-overall} $= 0$)} 
    \end{subfigure}
    \caption{Student \student's attempts synthesized by different methods instantiated from our framework for the scenario shown in Figure \ref{fig:python-problem-setup}. The student's misconception is: ``\textit{Time complexity is violated}''. For each method, we show the score of each attribute in the quality rubric. We highlight lines of code that reflect the student's misconception in \colorbox{pink}{pink}.} 
\end{figure}
